# Supplementary material for: JoyAI-Voice 2.0: A Full-Continuous Autoregressive Speech Generation Model with Semantic-Acoustic Joint Representation
Source: arXiv:2610.08834 source file (2026-09-29)
Supplement: Supplementary file 1 [file 99_appendix.tex]

\newpage
\section{Appendix}
\subsection{Training Data Example}
\begin{lstlisting}[language=json,caption={Example of monitoring and alerting.}, label={lst:example1}]
      {
        "role": "user",
        "content": "Alert me whenever a physical confrontation happens. \n<0.0 seconds>\n<image>\n<image>"
      },
      {
        "role": "assistant",
        "content": "</silence>"
      },
      {
        "role": "user",
        "content": "<1.0 seconds>\n<image>\n<image>"
      },
      {
        "role": "assistant",
        "content": "</silence>"
      },
      {
        "role": "user",
        "content": "<2.0 seconds>\n<image>\n<image>"
      },
      {
        "role": "assistant",
        "content": "</silence>"
      },
      {
        "role": "user",
        "content": "<3.0 seconds>\n<image>\n<image>"
      },
      {
        "role": "assistant",
        "content": "</silence>"
      },
      {
        "role": "user",
        "content": "<4.0 seconds>\n<image>\n<image>"
      },
      {
        "role": "assistant",
        "content": "</response> A physical confrontation is happening."
      },
      {
        "role": "user",
        "content": "<5.0 seconds>\n<image>\n<image>"
      },
      {
        "role": "assistant",
        "content": "</response> A physical confrontation is happening."
      },
      {
        "role": "user",
        "content": "<6.0 seconds>\n<image>\n<image>"
      },
      {
        "role": "assistant",
        "content": "</response> A physical confrontation is happening."
      },
      {
        "role": "user",
        "content": "<7.0 seconds>\n<image>\n<image>"
      },
      {
        "role": "assistant",
        "content": "</response> A physical confrontation is happening."
      },
      {
        "role": "user",
        "content": "<8.0 seconds>\n<image>\n<image>"
      },
      {
        "role": "assistant",
        "content": "</response> A physical confrontation is happening."
      },
      {
        "role": "user",
        "content": "<9.0 seconds>\n<image>\n<image>"
      },
      {
        "role": "assistant",
        "content": "</response> A physical confrontation is happening."
      },
      {
        "role": "user",
        "content": "<10.0 seconds>\n<image>\n<image>"
      },
      {
        "role": "assistant",
        "content": "</silence>"
      },
      ...
\end{lstlisting}

\newpage
\begin{lstlisting}[language=json,caption={Example of multi-turn casual chat.}, label={lst:example2}]
      ...
      {
        "role": "user",
        "content": "Is the person cleaning the desk?\n<7.0 seconds>\n<image>\n<image>\n<image>\n<image>"
      },
      {
        "role": "assistant",
        "content": "</response> Yep, definitely cleaning the desk! Getting all the dust off that pink surface."
      },
      {
        "role": "user",
        "content": "<8.0 seconds>\n<image>\n<image>\n<image>\n<image>"
      },
      {
        "role": "assistant",
        "content": "</silence>"
      },
      {
        "role": "user",
        "content": "<9.0 seconds>\n<image>\n<image>\n<image>\n<image>"
      },
      {
        "role": "assistant",
        "content": "</silence>"
      },
      {
        "role": "user",
        "content": "<10.0 seconds>\n<image>\n<image>\n<image>\n<image>"
      },
      {
        "role": "assistant",
        "content": "</silence>"
      },
      {
        "role": "user",
        "content": "<11.0 seconds>\n<image>\n<image>\n<image>\n<image>"
      },
      {
        "role": "assistant",
        "content": "</silence>"
      },
      {
        "role": "user",
        "content": "<12.0 seconds>\n<image>\n<image>\n<image>\n<image>"
      },
      {
        "role": "assistant",
        "content": "</silence>"
      },
      {
        "role": "user",
        "content": "What are they doing with the pillow?\n<13.0 seconds>\n<image>\n<image>\n<image>\n<image>"
      },
      {
        "role": "assistant",
        "content": "</response> They're picking up the pillow and moving it around, maybe fluffing it or putting it somewhere."
      },
      {
        "role": "user",
        "content": "<14.0 seconds>\n<image>\n<image>\n<image>\n<image>"
      },
      {
        "role": "assistant",
        "content": "</silence>"
      },
      {
        "role": "user",
        "content": "<15.0 seconds>\n<image>\n<image>\n<image>\n<image>"
      },
      {
        "role": "assistant",
        "content": "</silence>"
      },
      {
        "role": "user",
        "content": "<16.0 seconds>\n<image>\n<image>\n<image>\n<image>"
      },
      {
        "role": "assistant",
        "content": "</silence>"
      },
      {
        "role": "user",
        "content": "<17.0 seconds>\n<image>\n<image>\n<image>\n<image>"
      },
      {
        "role": "assistant",
        "content": "</silence>"
      },
      {
        "role": "user",
        "content": "Why is the person holding keys now?\n<18.0 seconds>\n<image>\n<image>\n<image>\n<image>"
      },
      {
        "role": "assistant",
        "content": "</response> Hmm, they seem to be fiddling with the keys on the desk. Maybe checking or organizing them?"
      },
      ...
\end{lstlisting}

\newpage
\begin{lstlisting}[language=json,caption={Example of background model delegation.}, label={lst:example3}]
      ...
      {
        "role": "user",
        "content": "<29.0 seconds>\n<image>\n<image>\n<image>\n<image>"
      },
      {
        "role": "assistant",
        "content": "</silence>"
      },
      {
        "role": "user",
        "content": "What are those two guys doing near the boat?\n<30.0 seconds>\n<image>\n<image>\n<image>\n<image>"
      },
      {
        "role": "assistant",
        "content": "</response> Looks like they're walking alongside it, probably supervising or guiding as it gets lifted."
      },
      {
        "role": "user",
        "content": "<31.0 seconds>\n<image>\n<image>\n<image>\n<image>"
      },
      {
        "role": "assistant",
        "content": "</silence>"
      },
      {
        "role": "user",
        "content": "<32.0 seconds>\n<image>\n<image>\n<image>\n<image>"
      },
      {
        "role": "assistant",
        "content": "</silence>"
      },
      {
        "role": "user",
        "content": "<33.0 seconds>\n<image>\n<image>\n<image>\n<image>"
      },
      {
        "role": "assistant",
        "content": "</silence>"
      },
      {
        "role": "user",
        "content": "<34.0 seconds>\n<image>\n<image>\n<image>\n<image>"
      },
      {
        "role": "assistant",
        "content": "</silence>"
      },
      {
        "role": "user",
        "content": "<35.0 seconds>\n<image>\n<image>\n<image>\n<image>"
      },
      {
        "role": "assistant",
        "content": "</silence>"
      },
      {
        "role": "user",
        "content": "<36.0 seconds>\n<image>\n<image>\n<image>\n<image>"
      },
      {
        "role": "assistant",
        "content": "</silence>"
      },
      {
        "role": "user",
        "content": "<37.0 seconds>\n<image>\n<image>\n<image>\n<image>"
      },
      {
        "role": "assistant",
        "content": "</silence>"
      },
      {
        "role": "user",
        "content": "Why does this boat hoist use a four-point sling configuration with spreader bars rather than lifting from a single central point, and how does the load distribution prevent hull deformation in fiberglass vessels?\n<38.0 seconds>\n<image>\n<image>\n<image>\n<image>"
      },
      {
        "role": "assistant",
        "content": "</response> Let me check the engineering principles behind that hoist design. </delegation> Explain the structural engineering principles of four-point boat lifting slings, load distribution, and hull deformation prevention in fiberglass boat hoists."
      },
      {
        "role": "user",
        "content": "<39.0 seconds>\n<image>\n<image>\n<image>\n<image>"
      },
      {
        "role": "assistant",
        "content": "</silence>"
      ...
\end{lstlisting}
